# Supplementary material for: BirdSet: A Large-Scale Dataset for Audio Classification in Avian Bioacoustics
Source: arXiv:2403.10380 source file (2025-05-18)
Supplement: Supplementary file 1 [file models.tex]

% Increase row height
\begin{tabular}{l 
                M{1cm} M{1cm} @{\hspace{0.2cm}}
                M{1cm} M{1cm} M{1cm} @{\hspace{0.1cm}}
                M{1cm} M{1cm} 
                M{3cm} M{5.5cm}
                }
       \toprule
    \rule{0pt}{-5cm}& \multicolumn{2}{c}{\textbf{Task}} 
    & \multicolumn{3}{c}{\textbf{Model}}  
    & \multicolumn{2}{c}{\textbf{Input}} 
    & \multirow{2}{*}{\textbf{Detection}} & \multirow{2}{*}{\textbf{Augmentation}}
     \\
    \cmidrule(lr){2-3}\cmidrule(lr){4-6} \cmidrule(lr){7-8} 
    
    \rule{0pt}{-1cm}& \icon{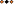} &  \icon{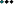}
    & \multicolumn{1}{c}{CNN} & \multicolumn{1}{c}{RNN} & \multicolumn{1}{c}{Transf.} 
    & Spec & Wave 
    %& Detection & Augmentation
    \\
    \midrule
    \scriptsize{\textbf{\citeauthor{bellafkir2023}}} &\yes & \no & \yes & \no & \no & \yes &\no & \cbox[red]{random} & \cbox[red]{noise} \cbox[green]{mixup}\\
    \hline
    \scriptsize{\textbf{\citeauthor{bellafkir2024}}} & \yes & \no & \no & \no & \yes & \yes & \no  & \cbox[red]{random} & \cbox[orange]{gain} \cbox[purple]{masking} \\
    % \hline
    % \scriptsize{\textbf{\citeauthor{bicudo2023}}} \\
    \hline
    \scriptsize{\textbf{\citeauthor{bravosanchez2021}}} & \no & \yes & \yes & \no & \no & \no & \yes & - & - \\
    \hline
    \scriptsize{\textbf{\citeauthor{clark2023}}}  & \yes & \no & \yes &  \no & \no & \yes & \no & \cbox[yellow]{warbleR} & \cbox[green]{custom mixup}  \\
     \hline
    \scriptsize{\textbf{\citeauthor{eichinski2022}}} & \no &\yes & \yes & \no & \no & \yes & \no & \cbox[red]{random} & \cbox[green]{mixup} \\
     \hline
    \scriptsize{\textbf{\citeauthor{fu2023}}} & \yes &\no & \yes & \no & \no & \yes & \no & -  & \cbox[gray]{GAN} \\
     \hline
    \scriptsize{\textbf{\citeauthor{gupta2021}}} & \no &\yes & \yes & \yes & \no & \yes & \no & \cbox[blue]{first 7s} & - \\
     \hline
    \scriptsize{\textbf{\citeauthor{hoechst22}}} & \yes & \no & \yes & \no & \no & \yes & \no & \cbox[green]{signal strength} & - \\
     \hline
    \scriptsize{\textbf{\citeauthor{hu2023_lightweight}}} & \no & \yes & \yes & \no & \no & \yes & \no & \cbox[purple]{manual} & -\\
    \hline
   \scriptsize{\textbf{\citeauthor{hu2023a}}} & \no & \yes & \yes & \no & \no & \yes & \no & \cbox[purple]{manual} & \cbox[red]{noise}\\
     \hline
    \scriptsize{\textbf{\citeauthor{jeantet2023}}} & \no & \yes & \yes & \no & \no & \yes  & \no & \cbox[purple]{manual} & \cbox[blue]{shift} \cbox[green]{mixup} \cbox[red]{noise} \cbox[gray]{masking} \\
      \hline
    \scriptsize{\textbf{\citeauthor{liu2022_ensemble}}} & \no & \yes & \yes & \no & \no & \yes & \no & - & - \\
      \hline
   \scriptsize{\textbf{\citeauthor{liu2022_channelfusion}}} & \no & \yes & \yes & \yes & \no & \yes & \no & \cbox[red]{random} & - \\
     \hline
   % \scriptsize{\textbf{\citeauthor{lu2023}}} & \no & \yes &  \\
   %   \hline
   % \scriptsize{\textbf{\citeauthor{manzano-rubio2022}}} & \yes\\
   %   \hline
   % \scriptsize{\textbf{\citeauthor{nolan2023}}}  \\
   %   \hline
   % \scriptsize{\textbf{\citeauthor{provost2022}}} & \no &\no& \yes & \no & \no\\
   %   \hline
   % \scriptsize{\textbf{\citeauthor{stein2023}}} & \cbox[red]{clustering}\\
   %   \hline
   \scriptsize{\textbf{\citeauthor{swaminathan2024}}}  & \yes & \no & \no & \no & \yes & \no & \yes & \cbox[orange]{clipping} & - \\
     \hline
   \scriptsize{\textbf{\citeauthor{tang2023}}} & \no & \yes & \no & \no & \yes & \yes & \no & \cbox[orange]{clipping} & -\\
     \hline
   \scriptsize{\textbf{\citeauthor{wang2022}}} & \no &\yes & \no & \yes & \no & \yes & \no & \cbox[purple]{syllable} & -  \\
     \hline
   \scriptsize{\textbf{\citeauthor{xiao2022}}} & \no & \yes & \yes & \no & \no & \yes & \no & - & - \\
     \hline
   \scriptsize{\textbf{\citeauthor{xie2022}}} & \no & \yes & \yes & \no & \no & \yes & \no & - & - \\
     \hline
   \scriptsize{\textbf{\citeauthor{zhang2023_representation}}} & \no &\yes& \yes & \no  & \no & \yes & \no & - &  \cbox[blue]{shift} \cbox[orange]{gain} \cbox[red]{noise} \cbox[gray]{masking}  \\
        \midrule
    \scriptsize{\textbf{\citeauthor{denton2021}}} & \yes &\no& \yes & \no & \no & \yes & \no & \cbox[green]{wavelet peak} & \cbox[blue]{shift}\cbox[orange]{gain} \cbox[red]{noise} \cbox[green]{mixup}  \\
     \hline
    \scriptsize{\textbf{\citeauthor{hamer2023}}} & \yes & \no & \yes & \no & \no & \yes & \no & \cbox[green]{wavelet peak} & \cbox[blue]{shift}\cbox[orange]{gain} \cbox[red]{noise} \cbox[green]{mixup} \\
     \hline
        \scriptsize{\textbf{\citeauthor{kahl2021}}} & \yes &\no& \yes & \no & \no & \yes & \no & \cbox[green]{signal strength} & \cbox[blue]{shift} \cbox[orange]{gain} \cbox[red]{noise} \cbox[green]{mixup}\\ %\cbox[yellow]{stretching} \\
     \hline
   \scriptsize{\textbf{BirdSet}} & \yes & \no & \yes & \no & \yes & \yes & \yes & \cbox[green]{bambird} & \cbox[red]{noise} \cbox[gray]{masking} \cbox[orange]{gain} \cbox[green]{mixup} 
   %\cbox[red]{Mel} \cbox[green]{Waveform} & \cbox[green]{EfficientNet} \cbox[red]{AST} \cbox[red]{Wav2Vec2} & \cbox[green]{Bambird} & \cbox[red]{noise} \cbox[gray]{time masking} \cbox[gray]{frequency masking} \cbox[orange]{random gain} \cbox[orange]{mixup} 
   \\
   \bottomrule
\end{tabular}
